# Supplementary material for: Regret and Conservatism of Distributionally Robust Constrained Stochastic Model Predictive Control
Source: arXiv:2309.12190 source file (2024-03-14)
Supplement: Supplementary file 1 [file appendix.tex]

%\section*{Appendix}
